# Supplementary material for: Differentially Private Online Learning
Source: arXiv:1109.0105 source file (2011-09-16)
Supplement: Supplementary file 1 [file supp.tex]

\subsection{ Sensitivity of IGD Algorithm} 
\label{sec:IGDSensitive} 

We present the proof of the bound on the sensitivity of our \igd\ algorithm here. 

\begin{lemma}[{\bf \igd\ Sensitivity}]
Sensitivity of the \igd\ algorithm is $\frac{2L}{t}$ for the $t$-th iterate, where $L$ is the maximum Lipschitz constant of any function $f_{\tau}, 1\leq \tau\leq t$. 
\label{lem:Sen}
\end{lemma}
\begin{proof}
We prove the above lemma using mathematical induction. \\
{\bf Base Case ($t=1$)}: As $\x_1$ is selected randomly, it's value doesn't depend on the underlying dataset. \\
{\bf Induction Step $t=\tau+1$}: As $f_\tau$ is $\alpha$ strongly convex. The total convexity of the function $$\tilde{f}_\tau(\x)=\frac{1}{2}\|\x-\x_{\tau}\|_2^2+\eta_\tau f_\tau(\x),$$ 
is $\frac{\tau+1}{\tau}$. Now using strong convexity and the fact that at optima $\x_{\tau+1}$,
$$\partial \tilde{f}_\tau(\x_{\tau+1}) (\x-\x_{\tau+1})\geq 0, \forall \x\in \C,$$
we get:
\begin{equation}
  \label{eq:sens_opt_r}
  \tilde{f}_\tau(\x_{\tau+1}')\geq \tilde{f}_\tau(\x_{\tau+1})+\frac{\tau+1}{2\tau}\|\x_{\tau+1}-\x_{\tau+1}'\|_2^2.
\end{equation}
Now, we consider two cases:
\begin{itemize}
\item {\bf $F-F'=\{f_\tau\}$}: Define $\tilde{f}_\tau'(\x)=\frac{1}{2}\|\x-\x_{\tau}\|^2+\eta_\tau f_\tau'(\x)$ and let $\x_{\tau+1}'=\argmin_{\x\in \C} \tilde{f}_\tau'(\x)$. Then, similar to \eqref{eq:sens_opt_r}, we get:
\begin{equation}
  \label{eq:sens_opt_rp1}
  \tilde{f}_\tau'(\x_{\tau+1})\geq \tilde{f}_\tau'(\x_{\tau+1}')+\frac{\tau+1}{2\tau}\|\x_{\tau+1}-\x_{\tau+1}'\|_2^2.
\end{equation}
Adding \eqref{eq:sens_opt_r} and \eqref{eq:sens_opt_rp1}, we get:
$$\|\x_{\tau+1}-\x_{\tau+1}'\|_2^2\leq \frac{1}{\tau+1}|f_\tau(\x_{\tau+1}')+f_\tau'(\x_{\tau+1})-f_\tau(\x_{\tau+1})-f_\tau'(\x_{\tau+1}')|\leq \frac{2L}{\tau+1}\|\x_{\tau+1}-\x_{\tau+1}'\|_2.$$
Lemma now follows using simplification. 
\item {\bf $F-F'=\{f_i\},\ i<\tau$}: Define $\tilde{f}_\tau'(\x)=\frac{1}{2}\|\x-\x_\tau'\|^2+\eta_\tau f_\tau(\x)$ and let $\x_{\tau+1}'=\argmin_{\x\in \C} \tilde{f}_\tau'(\x)$. Then, similar to \eqref{eq:sens_opt_r}, we get:
\begin{equation}
  \label{eq:sens_opt_rp11}
  \tilde{f}_\tau'(\x_{\tau+1})\geq \tilde{f}_\tau'(\x_{\tau+1}')+\frac{\tau+1}{2\tau}\|\x_{\tau+1}-\x_{\tau+1}'\|_2^2.
\end{equation}
Adding \eqref{eq:sens_opt_r} and \eqref{eq:sens_opt_rp11}, we get:
$$\|\x_{\tau+1}-\x_{\tau+1}'\|_2^2\leq \frac{\tau}{\tau+1}|(\x_{\tau+1}-\x_{\tau+1}')\cdot(\x_\tau-\x_\tau')|\leq \frac{\tau}{\tau+1}\|\x_{\tau+1}-\x_{\tau+1}'\|_2\|\x_{\tau}-\x_{\tau}'\|_2.$$
Lemma now follows after simplification and using induction hypothesis. 
\end{itemize}
\end{proof}

\subsection{Privacy Guarantee for Private Online Convex Programming}
\label{Sec:OCP1}
\label{sec:OCPPriv}
Note that every step of our private algorithm adds noise proportional to the sensitivity of the algorithm at that step to obfuscate the output, so as to provide privacy guarantee for that particular step. We make the claim precise in the following lemma. 
\begin{lemma}
Let $c>0$ be any constant, and $\beta=\lambda_\A T^{0.5+c}\sqrt{\frac{2}{\epsilon}\left(\ln\frac{T}{\delta}+\frac{\sqrt{\epsilon}}{T^{0.5+c}}\right)}$. Then step $t$ of algorithm~\ref{alg:ocp_diff}, i.e., $t$-th step output $\hatx_{t+1}$ is $(\frac{\sqrt\epsilon}{T^{0.5+c}},\frac{\delta}{T})$-differentially private.
\label{Lem:SingGenPriv}
\end{lemma}

\begin{proof}
As the output $\hatx_{t+1}$ is just a projection, i.e., a function (independent of the input functions $F$) of $\tx_{t+1}$, hence $(\epsilon, \delta)$-differential privacy for $\tx_{t+1}$ would imply the same for $\hatx_{t+1}$.
 
Now by the definition of differential privacy (see Definition~\ref{def:dp}), $\txt$ is $(\epsilon_1, \frac{\delta}{T})$-differential private, if for any measurable set $\Omega\subseteq\mathbb{R}^{p}$:
$$\Pr[\txt\in \Omega]\leq e^{\epsilon_1}\Pr[\txt'\in \Omega]+\delta/T,$$
where $\txt=\xt+b$ is the output of the noise additions step (see Algorithm~\ref{alg:ocp_diff}, Step 7) of our differentially private algorithm $\A_P$, when applied to function sequence $F_t=\langle f_1, \dots, f_t\rangle$. Similarly, $\txt'=\xt'+b$ is the output of the noise addition to $\xt'$ which is obtained by applying update step to $F_t'$ where $F_t'$ differs from $F_t$ in exactly one function entry. 

Now, $\txt\sim {\mathcal N}(\x_{t+1},\frac{\beta^2}{t^2} \mathbb{I}^d)$ and $\txt'\sim {\mathcal N}(\x_{t+1}', \frac{\beta^2}{t^2} \mathbb{I}^d)$. Hence:
\begin{eqnarray*}
\frac{\Pr[\txt\in \Omega]}{\Pr[\txt'\in \Omega]}=\frac{\int_{\x\in \Omega}\pdf(\txt=\x)}{\int_{\x\in \Omega}\pdf(\txt'=\x)}=\frac{\int_{\x\in \Omega}\exp\left(-\frac{\ltwo{\x-\xt}^2}{2\frac{\beta^2}{t^2}}\right)d\x}{\int_{\x\in \Omega}\exp\left(-\frac{\ltwo{\x-\xt'}^2}{2\frac{\beta^2}{t^2}}\right)d\x}
\end{eqnarray*}
%Let $b=\theta-\mathcal{M}_i(T_i)$, and $f=\mathcal{M}_i(T'_i)-\mathcal{M}_i(T_i)$. We have

Let $\dxt=\xt-\xt'$. Next, we bound each individual term in the above integration: 
\begin{align}
  \frac{\exp\left(-\frac{t^2 \ltwo{\x-\xt}^2}{2\beta^2}\right)}{\exp\left(-\frac{t^2\ltwo{\x-\xt'}^2}{2\beta^2}\right)}&=\exp\left(\frac{t^2}{2\beta^2}\dxt^T(2\x-\xt-\xt')\right),\nonumber\\
&=\exp\left(\frac{t^2}{2 \beta^2}\left(2\dxt^T(\x-\xt)-\|\dxt\|_2^2\right)\right), \nonumber\\
&\leq \exp\left(\frac{t^2}{2 \beta^2 }\left(2|\dxt^T(\x-\xt)|+\|\dxt\|_2^2\right)\right), \nonumber\\
&\leq \exp\left(\frac{t^2}{\beta^2}|\dxt^T(\x-\xt)|\right)\exp\left(\frac{\lambda_\A^2}{2\beta^2}\right), 
\label{eq:HPB}
\end{align}
where the last inequality follows from the sensitivity assumption~\eqref{eq:sens_ocp}. 

Since $\txt\sim\mathcal{N}(\xt,\frac{\beta^2}{t^2}\I_p)$, we have $(\txt-\xt)^T\dxt\sim\mathcal{N}(0,\frac{\beta^2}{t^2}\|\dxt\|_2^2)$. %Using the maximum value of $f$ (from the assumption on the sensitivity of $\mathcal{A}(T_i))$, we analyze the worst case,~\emph{i.e.,} we assume $\langle b,f\rangle\sim\mathcal{N}(0,\frac{\beta^2\lambda^2}{i^2})$. 
Now, using \eqref{eq:sens_ocp} and Mill's inequality, $$\Pr[|(\txt-\xt)^T\dxt|\geq \frac{\beta\lambda_\A}{t^2}z]\leq \Pr[|(\txt-\xt)^T(\dxt)|\geq\frac{\beta}{t}\|\xt-\xt'\|z]\leq e^{-\frac{z^2}{2}},$$ where $z>0$. Setting R.H.S. $\leq\frac{\delta}{T}$, we have $z\geq\sqrt{2\ln\frac{T}{\delta}}$. 

We call the set of $\txt\in \Omega$ to be the ``good set'' $\G$ if 
\begin{equation}
\label{eq:good}
(\txt-\xt)^T\dxt\geq\frac{\beta\lambda_\A}{t^2}z.
\end{equation}
Using the above bound, $\Pr[\txt\not\in \G]\leq \frac{\delta}{T}$ and for all $\x\in \G$:
\begin{align}
\exp\left(\frac{t^2}{\beta^2}|\dxt^T(\x-\xt)|\right)\exp\left(\frac{\lambda_\A^2}{2\beta^2}\right)&\leq \exp\left(\frac{\lambda_\A^2}{2\beta^2}+\frac{\lambda_\A}{\beta}\sqrt{2\ln\frac{T}{\delta}}\right),\nonumber\\
&\leq e^{\epsilon_1},
\label{eq:expupg}
\end{align}
where $\epsilon_1=\frac{\sqrt\epsilon}{T^{0.5+c}}$ and $\beta$ is as given in the Lemma statement. 

Similarly, we can define set $\G'$ for $\txt'$ and furthermore, 
\begin{equation}
  \label{eq:gg}
  \Pr[\txt\in\G]=\Pr[\txt'\in \G'].
\end{equation}
Combining \eqref{eq:HPB} and \eqref{eq:expupg}:
\begin{equation}
  \label{eq:ogog}
  \Pr[\txt\in\Omega|\txt\in \G]\leq e^{\epsilon_1}\Pr[\txt'\in \Omega|\txt'\in \G'].
\end{equation}
Using \eqref{eq:gg} and \eqref{eq:ogog}:
\begin{align}
  \Pr[\txt\in \Omega]&\leq \Pr[\txt\in \Omega|\txt\in \G]\Pr[\txt\in \G]+\Pr[\txt\not\in \G],\nonumber\\
& \leq e^{\epsilon_1} \Pr[\txt'\in \Omega|\txt\in \G]\Pr[\txt'\in \G]+\delta, \nonumber\\
& \leq e^{\epsilon_1} \Pr[\txt'\in \Omega]+\delta. 
\label{eq:txtx}
\end{align}
Hence, proved. 
\end{proof}

The above lemma shows $(\frac{\sqrt\epsilon}{T^{0.5+c}},\frac{\delta}{T})$-differential privacy for each step of the \ocp\ algorithm. To prove the privacy of our online Algorithm \ref{alg:ocp_diff} over {\em all} $T$-iterations we use the following lemma by \cite{DRV}. Our proof strategy from here on is inspired from a proof technique developed by \cite{HR}. 

\begin{lemma}[\cite{DRV}]
Suppose two random variables $Y$ and $Z$ satisfy $$D_\infty(Y||Z)=\max_{w\in\supp(Y)}\ln\left(\frac{\pdf[Y=w]}{\pdf[Z=w]}\right)\leq\epsilon,\ \ \ D_{\infty}(Z||Y)\leq\epsilon.$$ Then $D(Y||Z)=\int_{w\in\supp(Y)}\pdf[Y=w]\ln\left(\frac{\pdf[Y=w]}{\pdf[Z=w]}\right)\leq 2\epsilon^2$. Here $supp(Y)$ is the support set of a random variable $Y$.
\label{lem:Dwork}
\end{lemma}

We now state a technical lemma which will be useful for our privacy. 

\begin{lemma}
Assuming that at each stage $T$,  algorithm~\ref{alg:ocp_diff} preserves $\frac{\sqrt{\epsilon}}{T^{0.5+c}}$-differential privacy, $$\E_{ \txt}\left[\ln\left(\frac{\pdf[\txt]}{\pdf[\txt'=\txt]}\right)\right]\leq\frac{2\epsilon}{T^{1+2c}},$$
where $\txt$ and $\txt'$ are output of the $t$-th time step Noise Addition Step of our private ocp\ algorithm (Algorithm~\ref{alg:ocp_diff}), when applied to function sequences $F_t$ and $F_t'$ differing in exactly one function entry. 
\label{lem:pro}
\end{lemma}
\begin{proof}
Using the fact that $\txt$ is $\frac{\sqrt{\epsilon}}{T^{0.5+c}}$-differential private: 
$$\forall \x,\hspace{0.1cm}-\frac{\sqrt{\epsilon}}{T^{0.5+c}}\leq\ln\left(\frac{\pdf[\txt=\x]}{\pdf[\txt'=\x]}\right)\leq \frac{\sqrt{\epsilon}}{T^{0.5+c}}.$$
Lemma now follows using the above observation with Lemma~\ref{lem:Dwork}. 
\end{proof}
 
Finally, we state the privacy guarantee for algorithm~\ref{alg:ocp_diff} over all the $T$-iterations.
\begin{thm}[Privacy \ocp]
The Private \ocp\ algorithm (see Algorithm~\ref{alg:ocp_diff}) is $(3\epsilon,2\delta)$-differentially private.
\label{Thm:GenPri}
\end{thm}

\begin{proof}
Following the notation from the proof of lemma~\ref{Lem:SingGenPriv} we define the ``good'' set $\G$ (see \eqref{eq:good}). Now, using \eqref{eq:gg} and Lemma~\ref{Lem:SingGenPriv}, for each round, 
\begin{equation}
\Pr[\txt\in\G]=\Pr[\txt'\in \G']=\frac{\delta}{T}.   
\end{equation}
Now, probability that the noise vector $\b=\txt-\xt=\txt'-\xt'$ always leads to ``good'' set in all $T$ rounds is $T\cdot \frac{\delta}{T}=\delta$. 

Now, we condition the remaining proof on the fact that the noise vector $\b$ in each round is such that $\tx_t\in \G$ and $\tx_t'\in \G'$. 

Let $L(\tx_1,\cdots,\tx_T)=\sum_{t=1}^T\ln\left(\frac{\pdf(\tx_t)}{\pdf(\tx_t'=\tx_t)}\right)$, where each $\x_t\in\mathbb{R}^d$.

Therefore, by Lemma~\ref{lem:pro}, $$\E[L(\tx_1,\cdots,\tx_T)]=\sum_{t=1}^T \E_{\tx_t}\left[\ln\left(\frac{\pdf(\tx_t)}{\pdf(\tx_t'=\tx_t)}\right)\right]\leq \frac{2T\epsilon}{T^{1+2c}}\leq\frac{2\epsilon}{T^{2c}}\leq 2\epsilon.$$

Let $Z_t=\ln\left(\frac{\pdf(\tilde{x}_t=\xt)}{\pdf(\tilde{x}_t'=\x_t)}\right)$. Since the randomness is freshly added in each iteration, $Z_t$ are independent. We have $L(\x_1,\cdots,\x_T)=\sum_{t=1}^T Z_t$, where $|Z_t|\leq\frac{\sqrt{\epsilon}}{T^{0.5+c}}$. By Azuma-Hoeffding's inequality
\begin{align*}
\Pr[L(\tx_1,\cdot,\tx_T)\geq 2\epsilon+\epsilon]&\leq 2\exp\left(\frac{-2\epsilon^2}{T\times\frac{\epsilon}{T^{1+2c}}}\right),\\
&\leq 2\exp\left(-2T^{2c}\right).
\end{align*}
Let $\delta=2\exp\left(-2T^{2c}\right)$. We have $-2T^{2c}=\ln\frac{\delta}{2}$. Solving for $c$ we get $c=\frac{(\ln (\frac{1}{2}\ln \frac{2}{\delta} )}{2\ln T}$.

Hence, with probability $1-\delta$, $3\epsilon$-differential privacy holds conditioned on $\tx_t\in\G$ and $\tx_t'\in\G'$, i.e, 
$$\forall\x, \hspace{0.1cm}\Pi_{t=1}^T\pdf(\x_t=\x)\leq e^{3\epsilon}\Pi_{t=1}^T\pdf(\tx_t'=\x).$$
Also, recall that with probability $1-\delta$, our noise vector $\b$ in each round itself was such that $\tx_t\in \G$ and $\tx_t'\in \G'$. Theorem now follows using an argument similar to \eqref{eq:txtx}. 
\end{proof}

\subsection{Generic Regret Bound Analysis for OCP}
\label{sec:OCPReg}
In this section, we provide a generic regret bound analysis for Algorithm \ref{alg:ocp_diff}. The regret of our private \ocp\ algorithm depends on the regret $\R_\A(T)$ the non-private learning algorithm $\A$.

\begin{thm}[Regret Bound]
Let $L>0$ be the maximum Lipschitz constant of any function $f_t$ in the sequence $F$, %and let $\alpha>0$ be the minimum strong convexity parameter of any function $f_t$ in $F$. 
 and let the regret of the non-private \ocp\ algorithm $\A$ over $T$-time steps is $\R_{\A}(T)$ and let $\lambda_\A$ be the sensitivity parameter of $\A$ (see \eqref{eq:sens_ocp}), then the expected regret of our Private \ocp\ algorithm (Algorithm~\ref{alg:ocp_diff}) follows:
$$\E\left[\sum_{t=1}^Tf_t(\hat\x_t)\right]-\min_{\x\in\C}\sum_{t=1}^Tf_t(\x)\leq 2dL\lambda_\A\sqrt{T}\frac{\ln^2\frac{T}{\delta}}{\sqrt{\epsilon}}+\R_{\A}(T),$$  
%is upper bounded by 
%$$\R_{\A}(T)+\lambda_\A \sqrt{T\ln\sqrt{\frac{2}{\delta}}}\sqrt{\frac{2}{\epsilon}\left(\ln\frac{T}{\delta}+\frac{\sqrt{\epsilon}}{\sqrt{T\ln\sqrt{\frac{2}{\delta}}}}\right)}\left(\frac{\sqrt{2}\Gamma((d+1)/2)\ln T}{\Gamma(d/2)}\right),$$
where $d$ is the dimensionality of the output space. That is, the regret bound is $ R_\A(T)+\tilde{O}\left(d\sqrt{T}\right)$. 
\label{thm:util}
\end{thm}  

\begin{proof}
Let $\hat\x_1,\cdots,\hat  \x_T$ be the output of the POCP algorithm~\ref{alg:ocp_diff}. By the Lipschitz continuity of the cost functions $f_t$ we have
\begin{eqnarray}
&&\sum_{t = 1}^T f_t(\hat{\x}_t)-\min_{\x\in\C}\sum_{t=1}^Tf_t(\x) \leq \sum_{t = 1}^T f_t(\x_t)-\min_{\x\in\C}\sum_{t=1}^Tf_t(\x) + L \sum_{t = 1 }^T \ltwo{\hat{\x}_t - \x_t}\\
&&= R_\A(T) +  L \sum_{t = 1 }^T \ltwo{\hat{\x}_t - \x_t}.
\label{eq:rahx}
\end{eqnarray}
Since at any time $t$,  $\hat\x_{t}$ is the projection of $\tilde\x_{t}$ on the convex set $\C$, we have $$\ltwo{\x_t-\hat\x_t}\leq\ltwo{\x_t-\tilde{\x}_t}=\ltwo{\b_t},$$ where $\b_t$ is the noise vector added at in the $t^{th}$ iteration of algorithm~\ref{alg:ocp_diff}. Therefore,
\begin{equation} 
\sum_{t=1}^T L \ltwo{\x_{t}-\hat\x_{t}}\leq L \sum_{t =1}^T\ltwo{\b_{t}}.
\label{eq:hxb}
\end{equation}
Now, $\b_{t} \sim \mathcal{N} ( \0^d, \frac{\beta^2}{t^2} \I^d) $ where $$\beta= \lambda_{\A}T^{0.5+c}\sqrt{\frac{2}{\epsilon}\left(\ln\frac{T}{\delta}+\frac{\sqrt{\epsilon}}{T^{0.5+c}}\right)}.$$
 
Therefore, $\ltwo{\b_{t}}$ follows Chi-distribution with parameters $\mu=\frac{\sqrt{2}\frac{\beta}{t} \Gamma((d+1)/2)}{\Gamma(d/2)}$ and $\sigma^2=\frac{\beta^2}{t^2}(d-\mu^2)$. 

Using $c = \frac{\ln{ (\frac{1}{2}\ln{\frac{2}{\delta}})} }{2\ln{T}}$,
\begin{align}
 \E[\sum_{\tau=1}^T\ltwo{\b_{\tau}}] &\leq \frac{\sqrt{2}\beta \Gamma((d+1)/2)}{\Gamma(d/2)} \int_{\tau =1}^T \frac{1}{t}d\tau, \nonumber\\
&= \frac{\Gamma((d+1)/2)}{\Gamma(d/2)} \lambda_\A\sqrt{T}\ln {T}\sqrt{\frac{2}{\epsilon}\ln{\frac{2}{\delta}}\left(\ln\frac{T}{\delta}+\frac{\sqrt{\epsilon}}{\sqrt{\frac{T}{2}\ln{\frac{2}{\delta}}}}\right)},\nonumber\\
&\leq 2d\lambda_\A\sqrt{T}\frac{\ln^2\frac{T}{\delta}}{\sqrt{\epsilon}}. 
\label{eq:noisenorm}
\end{align}
The theorem now follows by combining \eqref{eq:rahx}, \eqref{eq:hxb}, \eqref{eq:noisenorm}. 
\end{proof}

%%% Local Variables: 
%%% mode: latex
%%% TeX-master: "nips2011"
%%% End: 

\section{Follow the Leader}
\label{sec:FTL}
As another application of Algorithm \ref{alg:ocp_diff} we describe our Private Follow The Leader Algorithm (\pftl). It is based on the Follow The Leader algorithm (\ftl\,) by \cite{HKKA}. \ftl\, at each time step $t+1$ outputs $\x_{t+1}=\argmin_{\x\in\C}\frac{1}{t}\sum_{\tau=1}^t f_{\tau}(\x)$. The first vector $\x_1\in\C$ is chosen  arbitrarily without querying the data set.  For \pftl\ we instantiate the non-private algorithm $\A$ (in Algorithm \ref{alg:ocp_diff}) with the following. Let $\mathcal{A}(F_t)=\argmin_{\x\in\C}\frac{1}{t}\sum_{\tau =1}^t f_{\tau}(\x)$, where $F_t=\langle f_1,\cdots,f_t\rangle$. We assume the following regarding the cost functions.
\begin{enumerate}
	\item The cost function $f_t(\x)$ can be written as $g_t(\langle \bm v_t,\x\rangle)+\frac{\alpha}{2}\ltwo{\x}^2$, where $g_t:\mathbb{R}\rightarrow\mathbb{R}$ is a univariate function and $\bm v_t$ is a vector s.t. $\ltwo{\bm v_t}\leq R$ (a constant). We need this condition for our regret bound.
	\item The cost function $f_t(\x)$ is $L$-Lipschitz in $\x$,~\emph{i.e.,} $|f_t(\x_1)-f_t(\x_2)|\leq L\ltwo{\x_1-\x_2},\forall \x_1,\x_2\in \C$.
	\item A relatively mild assumption is that the \emph{origin} ($\0^d$) is contained in the convex set $\C$.
\end{enumerate}

Our first lemma is about bounding the sensitivity of $\mathcal{A}(F_t)$.

\begin{lemma}
$L_2$-sensitivity of $\x_{t+1}=\argmin_{\x\in\C}\frac{1}{t}\sum_{\tau =1}^t f_{\tau}(\x)$ is $\frac{2L}{t\alpha}$.
\end{lemma}

\begin{proof}
$\x_{t+1}=\arg\min_{\x\in\C}\frac{1}{t}\sum_{\tau =1}^t f_{\tau}(\x)$ is the result of a constrained convex optimization on the convex set $\C$. For the ease of representation let $G_{t}(\x)=\frac{1}{t}\sum_{\tau=1}^t f_{\tau}(\x)$ . Let $G_t'$ be another summation where $G_t$ and $G_t'$  differ in exactly one of it summands. Let $\x'_{t+1}\in\C$ be the vector that minimizes $G'_{t}$.

For all points $y\in\C$, the following are true,
\begin{enumerate}
	\item $\subg{G_{t}}(\x_{t+1})^T(y-\x_{t+1})\geq 0$
	\item $\subg{G'_{t}}(\x'_{t+1})^T(y-\x'_{t+1})\geq 0$
\end{enumerate}
where $\subg{}$ is any subgradient of the function $G_t$ or $G_{t'}$.
The cost functions  $f_t$ are assumed to be $\alpha$-strongly convex. Thus, both $G_{t}$ and $G'_{t}$ are $\alpha$-strongly convex.
Thus, we have
\begin{eqnarray*}
&&G_t(\x'_{t+1})\geq G_t(\x_{t+1})+\frac{\alpha}{2}\ltwo{\x'_{t+1}-\x_{t+1}}^2\\
&&G'_t(\x_{t+1})\geq G'_t(\x'_{t+1})+\frac{\alpha}{2}\ltwo{\x'_{t+1}-\x_{i+1}}^2\\
\end{eqnarray*}
Combining the above two equations we have,
$$\alpha\ltwo{\x'_{t+1}-\x_{t+1}}^2\leq (G_t(\x'_{t+1})-G'_t(\x'_{t+1}))+(G'_t(\x_{t+1})-G_t(\x_{t+1}))$$
Let the summands of $G_t$ and $G'_k$ differ at position $k$. Therefore, $G_t(\x'_{t+1})-G'_t(\x'_{t+1})=\frac{1}{t}(f_k(\x'_{t+1})-f'_k(\x'_{t+1}))$ and $G'_t(\x_{t+1})-G_t(\x_{t+1})=\frac{1}{t}(f'_k(\x_{t+1})-f'_k(\x_{t+1}))$.
where $f'_k$ is another function differing from $f_k$.
Hence,
\begin{eqnarray}
&&\alpha\ltwo{\x'_{t+1}-\x_{t+1}}^2\leq\frac{1}{t}\left(f_k(\x'_{t+1})-f'_k(\x'_{t+1})+f'_k(\x_{t+1})-f_k(\x_{t+1})\right)\\
&&\leq \frac{2L}{t}\ltwo{\x'_{t+1}-\x_{t+1}}
\end{eqnarray}
The last inequality follows from the Lipschitz property of the cost function $f_t$.
Finally,
$$\ltwo{\x'_{t+1}-\x_{t+1}}\leq \frac{2L}{t\alpha}$$
\end{proof}

We fix $\lambda_\mathcal{A}=\frac{2L}{\alpha}$ in Algorithm~\ref{alg:ocp_diff} as the sensitivity parameter.

\begin{corollary}[Privacy]
Private \ftl\, is $(3\epsilon,2\delta)$-differentially private.
\end{corollary}
The proof of this corollary follows directly from Theorem \ref{Thm:GenPri}.

Before we state the regret bound for \pftl, we state the following theorem bounding the regret for non-private \ftl\, (\ie when we do not add noise to the output).  The proof can be obtained (with minor modification) from the regret bound analysis of the version of \ftl\, by  \cite{HAS}.

\begin{thm}[Regret bound for \ftl\,]
Assume that for all $t$, the function $f_t(x)$ can be written as $g_t(\langle v_t,\x\rangle)+\frac{\alpha}{2}\ltwo{\x}^2$ for a univariate convex function $g_t(\langle v_t,\x\rangle)$ and some vector $v_t\in\mathbb{R}^p$. Assume that for some $R,G >0$, we have $\ltwo{v_t}\leq R$ and for all $\x\in\C$, we have $| g'_t(\langle v_t,\x\rangle)|\leq G$ and $|g''_t(\langle v_t,\x\rangle)|\geq 0$. Also assume that the convex set $\C$ contains the origin. The  non-private \ftl\, over $T$ rounds has~\emph{regret}
$$\leq \frac{1}{\alpha}\left(G\ R+C\alpha\right)^2\ln T$$
where $C$ is the diameter of the convex set $\C$.
\label{Thm:UtilKalai}
\end{thm}

We now state the regret bound for \pftl. It follows as a corollary from Theorem~\ref{thm:util}.

\begin{corollary}[Regret bound for \pftl\,]
Suppose for all $t$, $f_t$ satisfies all the conditions in theorem  \ref{Thm:UtilKalai} Let the Lipschitz constant of $f_t$ for all $t$ be at most $L$. Then, the expected regret (\emph{i.e.,} $\E[\sum_{t=1}^Tf_t(\hat\x_t)]-\min_{\x\in\C}\sum_{t=1}^T f_t(\x))$  is upper bounded by
$$\frac{1}{\alpha}\left(\left(G R+C\alpha\right)^2\ln T+4\sqrt{d} L^2\sqrt{T}\frac{\ln^2\frac{2}{\delta}}{\sqrt \epsilon}\right)$$
where $C$ is the diameter of the convex set $\C$ and $d$ is the dimensionality of the output space.
\end{corollary} 
\input{giga}
\subsection{ FTL for Quadratic Costs} 
\label{sec:logRegret}
We prove the privacy and utility guarantees for our private FTL algorithm with Quadratic Cost functions here.
\begin{thm}
Let $f_t =\frac{1}{2} (y_t - \v_t^T\x)^2 + \frac{\alpha}{2}\ltwo{\x}^2$ for each $t$ be Lipschitz continuous with parameter $L$. For $\hat{\x}_t$  the output of the private FTL algorithm as in Algorithm \ref{Algo:quad} , and $\x_t$ the corresponding output of the non-private FTL, we have, with high probability,  $$\R_{privacy} = \sum_{t = 1 }^T ( f_t(\hat{\x}_t) - f_t(\x_t) ) = O( L^2 R^2d^2 \frac{1}{\sqrt{\epsilon}} \log^{1.5}{T} \log{\sqrt{\frac{\log{T}}{\delta}}} ) $$ 
\end{thm}
\begin{proof}
Using Lipschitz continuity of functions $f_1,\dots, f_t$ , 
\begin{align}
\R_{privacy} =  \sum_{t = 1} ^{T} ( f_t(\hat{\x}_t) - f_t(\x_t) )\leq L \sum_{t = 1} ^{T}  \ltwo{\hat{\x}_{t+1} - \x_{t+1} }   \label{eqnpriv}
\end{align}
We now bound $ \ltwo{\hat{\x}_{t+1} - \x_{t+1} }$. Let $\hat{V}_t = V_t + A_t$ and $\hat{\K}_t = \K_t + \N_t$  where $A_t$ and $\N_t$ are the noise additions introduced by the Private Partial sum Computing algorithm \ref{Algo:partialSum}.

From the Update Equation \eqref{eqnref:QuadUpdate} we have
\begin{align}
(\hat{V}_{t} + t\alpha \I ) \hat{\x}_t =  \hat{K}_t\quad \Leftrightarrow\quad (\frac{1}{t}\hat{V}_{t} + \alpha \I )\hat{x}_t &= \frac{1}{t} \hat{\K}_t  \label{eqnprav1}
\end{align}
Similarly for the non-private FTL's update equation we have, 
\begin{align}
(\frac{1}{t} V_t + \alpha \I) \x_t &= \frac{1}{t}\K_t \label{eqnprav2}
\end{align}
By combining \eqref{eqnprav1} and \eqref{eqnprav2}, we get:

$$ (\frac{1}{t}\hat{V}_{t} + \alpha \I )( \hat{\x}_t -\x_t) = \frac{1}{t} \N_t - \frac{1}{t}A_t\x_t $$
By triangle inequality we have,
\begin{equation}
\ltwo{ (\frac{1}{t}\hat{V}_{t} + \alpha \I )( \hat{\x}_t -\x_t) }  \geq \ltwo{ (\frac{1}{t}V_{t} + \alpha \I )( \hat{\x}_t -\x_t) } - \ltwo {  \frac{1}{t} A_t( \hat{\x}_t -\x_t)  }
\label{eq:Afbcs1}
\end{equation}
Now, the spectral norm $\ltwo{A_t}$ of $A_t$ satisfies, $\ltwo{A_t} \leq \lfrob{A_t}$. Furthermore, using Cauchy Schwartz inequality:
 \begin{align}
\ltwo {  \frac{1}{t} A_t( \hat{\x}_t -\x_t)  } &\leq \frac{1}{t} \ltwo{A_t}\ltwo{\hat{\x}_t - \x_t } \leq  \frac{1}{t} \lfrob{A_t}\ltwo{\hat{\x}_t - \x_t }
\label{eq:Afbcs}
\end{align}
Thus by combining \eqref{eq:Afbcs1}, \eqref{eq:Afbcs} and using the fact that the spectral norm of $(\frac{1}{t}V_{t} + \alpha \I)$ is lower-bounded by $\alpha$, 
\begin{align}
 (\alpha - \frac{\lfrob{A_t}}{t} ) \ltwo{\hat{\x}_t - \x_t }&\leq  \frac{1}{t}\ltwo{ \N_t} + \frac{1}{t}\ltwo{A_t\x_t}\label{eq:Afbcs3}
\end{align}
Now, each entry of the matrix $A_t$ is drawn from $\mathcal{N}( 0, \sigma^2)$ for $\sigma^2 = \frac{R^2}{\epsilon}\log{T}\log{\frac{\log{T}}{\delta}}$. Thus the spectral norm of $A_t$, $\ltwo{A_t}$ is a sum of independent Gaussian random variables and itself follows the Gaussian distribution with the variance multiplied. Hence by definition,  $\lfrob{A_t}$ follows Chi distribution with mean $\mu = \frac{\sqrt{2}\sigma\Gamma{(d^2+1)/2}}{\Gamma({d^2/2})}$ and Variance $\sigma^2 ( d^2 - \mu^2)$. Thus, with high probability 
 %(replace with an exact value here ? ) 
  $$\lfrob{A_t} \leq \sqrt{2}\sigma d^2+ \sigma d.$$
 Similarly, $\ltwo{\N_t} \leq \sqrt{2}\sigma d + \sigma \sqrt{d} $. Also, $\x_t = (\frac{1}{t}V_t + \alpha \I^d)^{-1} K_t$ Thus $\ltwo{\x_t} \leq R$ Using the above observation with \eqref{eq:Afbcs3}, 
 \begin{align*}
 \ltwo{\hat{\x}_t - \x_t } &\leq  \frac{1}{t}\cdot\frac{\ltwo{ \N_t} + \ltwo{A_t\x_t}}{\alpha - \frac{\lfrob{A_t}R}{t}}\leq \frac{O(\sigma R d^2)}{t}. 
%\leq \frac{1}{t}\cdot\frac{2\sqrt{2}Rd + 2\sigma Rd}{\alpha}=
 \end{align*}
Summing the above equation over $t=1$ to $T$:
 \begin{align*}
 \sum_{\tau = 1}^t \ltwo{\hat{\x}_{t+1} - \x_{t+1} } \leq \int_{\tau = 1 }^{T} \frac{O(\sigma R d^2)}{\tau} d\tau= O(\sigma R d^2)\log{T}= O( R^2 d^2 \frac{1}{\sqrt{\epsilon}} (\log{T})^{1.5} \log{\sqrt{\frac{log{T}}{\delta}}} ).
 \end{align*}
 The result now follows by using the above bound with \eqref{eqnpriv}. 
\end{proof}

\subsection{ Computing Partial Sums Privately }
\label{sec:partialSum}

In this section we generalize a technique proposed in \cite{DNPR} to compute partial sums for real vectors arriving online when each vector belongs to a different party. Differential Privacy of the algorithm guarantees that under an adversarial modification of one of the vectors, the sums output by the algorithm remain {\it almost} invariant. Thus the adversary cannot extract information about any particular party from the output of the algorithm.We use this algorithm as a black box to guarantee the privacy of our QPFTL algorithm.

We begin this section with a brief description of the algorithm and then show the privacy guarantees. 

For simplification of exposition we assume that $T = 2^k$ for some positive integer $k$. We compute a binary tree $\B$ of partial sums with leaves as the input vectors arriving online. Each node in the tree represents the sum of the vectors in the subtree rooted at the node. To represent this, we label the node at some level $i$ with strings in $\{0,1\}^{i}$. (The root is labeled with the empty string $\empty$) A node labeled with a string $s$ of length $i$ represents the privately computed partial sum  

$$\hat{\B}_s = \sum_{\begin{subarray}{c}j: \text{string}(j)  = s\circ t\\ t \in \{0,1\}^{k-i}\end{subarray} } \uu_j$$ where string(j) is the bit string representation of $j$ in $\{0,1\}^k$ and $\circ$ is the concatenation operation on strings.

Note that for this technique to work, we need to know the number of arriving values, $T$ in advance. We create a node in the tree only when all the vectors that form the leaves of the subtree rooted at the node have arrived. At time instant $\tau$ we receive vector $u_{\tau}$ and create the nodes which can now be created bottom up. Whenever we add a node, we compute the value to be stored at the node by summing up the values at its two children and adding a Gaussian noise of $0$ mean and appropriately computed variance.

To output the partial sum at an instant $\tau$, we express the sum in the form of sum of values at nodes in the tree, where we choose the nodes at the higher levels first.
\begin{algorithm}
	\caption{Private Partial Sum($\{\uu_i\}$, $\epsilon$, $\delta$, $R \geq max_{i \leq T} \ltwo{\uu_i} $ ) }
	\begin{algorithmic}[1]
		\REQUIRE Data vectors $\uu_i$ arriving online, privacy parameters $\epsilon$ and $\delta$,  $R$, and dimension of the vectors $d$
		\STATE Set $ \sigma^2 \leftarrow \frac{R^2}{\epsilon'} \log{T}\log{\frac{\log{T }}{\delta'}}$ where $\epsilon' = \frac{\epsilon}{d}$ and $\delta' = \frac{\delta}{d}$
		\STATE Initialize Binary Tree $\B$ and define $B_s$ and $\hat{\B}_s$ to be the exact and the noisy versions of the value at node labeled $s$.
		%\STATE Initialize $sum \leftarrow 0$
		%\STATE {\bf Segments}. For $i \in \{1, . . . , log T \}$, associate with each string $s \in \{0, 1\}^i$  the time segment $S$ of $2^{log T - i}$ time periods
%$\{s \circ 0^{logT- i},...s \circ 1^{logT - i}\}$. The segment begins in time $s\circ 0^{logT - i}$ and ends in time $s \circ 1^{logT - i}$
		%\STATE For each node (with label $s$ say) sample $\zeta_S \sim \mathcal{N}(0, \sigma^2)$
		\FOR{$\tau = 1$ to $T$} 
			\STATE $sum = sum + \uu_{\tau}$
			\STATE Let $s_{\tau}$ be the string representation of $\tau$ in binary.
			\STATE Create all nodes in the tree whose labels are $s$ such that $s_{\tau} = s\circ t$ and $t = 1^{c}$ for some $c < k$. 
			\STATE Initialize each of the nodes created with for $i\leq d$ $\bm{\zeta}_s(i) = \mathcal{N}(0,\sigma^2)$
			\STATE Update the value at each node $s$ created :\\$\hat{B}_s \leftarrow B_s + \bm{\zeta_s}$\\ $B_s \leftarrow B_s + B_{s\circ 0} + B_{s\circ 1}$
			\STATE Let $s_1, s_2,... ,s_{\log {T}}$ be the ${\log{T}}$ labels such that each $s_i$ is a prefix of $s_{\tau}$ \label{line:addNoise}
			\STATE {\bf Output:} $Sum_i = sum+\sum_{i=1}^{\log{T}}\hat{B_{s_i}} $
		\ENDFOR					
	\end{algorithmic}
	\label{Algo:partialSum}
\end{algorithm} 

\begin{thm}[Privacy] \label{PartialSumPrivacy}
Let $R \geq max_{i \leq T}\ltwo{\uu_i} $ and $ \sigma^2 = \frac{R^2}{\epsilon'} \log{T}\log{\frac{\log{T }}{\delta'}}$  where $\epsilon' = \frac{\epsilon}{d}$ and $\delta' = \frac{\delta}{d}$. Then the Private Partial Sum algorithm when run with the parameters $(\epsilon, \delta, R) $ outputs every partial sum with a random Gaussian error of  $\mathcal{N}(0, \sigma_{cum}^2)$ in every entry of the output vector where $\sigma_{cum} \leq \sigma\cdot \log{T}$  and enjoys $(\epsilon, \delta)$-differential privacy against a single intrusion.
\end{thm}

\begin{proof}
Line \ref{line:addNoise} of the algorithm adds at most $\log{T}$ vectors all of which have each of their entries chosen from an independent Gaussian distribution (noise)$ \mathcal{N}(0, \sigma^2)$. Since each of these random variables is independent, each entry in the output vector has a random Gaussian error of  $\mathcal{N}(0, \sigma_{cum}^2)$ where $\sigma_{cum} \leq \sigma\cdot \log{T}$.

If every entry of a vector of dimension $d$ is $(\frac{\epsilon}{d}, \frac{\delta}{d})$ differentially private then the vector itself is $(\epsilon, \delta)$ differentially private. Thus, without loss of generality we assume that $d =1 $ and proceed with the proof. 

To prove the differential privacy for any partial sum output by the algorithm, we show that at all times the values stored in the tree $B$ are differentially private. The partial sum returned by the algorithm at time $\tau$ is a function of the values stored at any of the existing nodes of the binary tree $B$ at $\tau$. The privacy guarantees for the partial sums then follows from the preservation of differential privacy under compositions. 

For the purpose of privacy guarantees, the Binary tree $\B$ can be seen as a vector of at most $2T-1$ values stored at its nodes. We refer to this vector as $\B$.
  Let $B_{s_1}, B_{s_2}, ..., $ be an arbitrary ordering of the nodes of $B$

 Let $\u$ and $\u'$ be two sets of inputs to the algorithm differing in exactly one entry, say at time $\tau$. Let the binary tree vectors produced in the two runs of the algorithm be $\B(\u)$ and $\B(\u')$ respectively. Consider          

\begin{claim}\label{claimBTree}
Suppose for any node $B_s$ at time $\tau$, $\Pr_{B^*_{s}} [e^{-\frac{\epsilon}{\log{T}} }  \leq \frac{ \Pr [ B_{s}(\u) = B^*_{s}]}  { \Pr[ B_{s_1}(\u') = B^*_{s}]}  \leq e^{\frac{\epsilon}{\log{T}} } ] \geq 1 - \frac{\delta}{\log{T}} $. Then $\B$ is $(\epsilon, \delta)$ differentially private at time $\tau$. 
\end{claim}
We first show how the claim implies the theorem. We then prove the claim and complete the proof.
Now, $$\frac{\Pr [ \B(\u) \in  S]}{\Pr [\B(\u') \in S]} =  \frac{\int_{\B^* \in S}\Pr [ \B(\u) = \B^*]}{\int_{\B^* \in S} \Pr [\B(\u') \in \B^*]} $$
\begin{align*}
\frac{ \Pr [ \B(\u) = \B^*]}  { \Pr [\B(\u') \in \B^*]}  &=  \frac{ \Pr [ B_{s_1}(\u) = B^*_{s_1}]} { Prob B_{s_1}(\u') = B^*_{s_1}]}  \frac{ \Pr [ B_{s_2}(\u) = B^*_{s_2} |  B_{s_1}(\u) = B^*_{s_1}]}  { Prob B_{s_1}(\u') = B^*_{s_1}   |  B_{s_1}(\u') = B^*_{s_1}] }\cdots\\
&= \frac{ \Pr [ B_{s_1}(\u) = B^*_{s_1}]} { \Pr[ B_{s_1}(\u') = B^*_{s_1}]}  \frac{ \Pr [ B_{s_2}(\u) = B^*_{s_2}]}  { \Pr[ B_{s_1}(\u') = B^*_{s_1} ] }\cdots\\
&\text{(follows from the independence of every noise vector added)}
\end{align*}
 Since $\u$ and $\u'$ differ in exactly one entry, $B(\u)$ and $B(\u')$ can differ in at most $\log{T}$ nodes. Thus at most $\log{T}$ ratios in the above product can be different from $1$. Thus by using the Claim and a Union Bound over the at most $\log{T}$ nodes which have differing values in $B(\u)$ and $B(\u')$, we have 
$$\Pr [e^{-\epsilon} \leq \frac{ \Pr [ \B(\u) = \B^*]} { \Pr [\B(\u') \in \B^*]}  \leq e^{\epsilon}] \geq 1 - \sum \frac{\delta}{\log{T}} = 1 - \delta$$
Thus , 
$$ \frac{ Pr [ \B(\u) = \B^*]}  { \Pr [\B(\u') = \B^*]}  \leq e^{-\epsilon } ( 1- \delta) + \delta \leq e^{\epsilon} + \delta $$ 
We now show the validity of the claim and complete the proof.

\begin{proof}[Proof of Claim \ref{claimBTree}]
Let $\Delta = B_s(\u) - B_s(\u')$
\begin{align*}
 \frac{ \Pr [ B_{s}(\u) = B^*_{s}]}  { \Pr [B_{s}(\u') = B^*_{s}]} &= \frac { \exp{\frac{\ltwo{B^*_s - B_s(\u)  }^2)}{2\sigma_{cum}^2}}}{ \exp{\frac{\ltwo{B^*_s - B_s(\u')  }^2)}{2\sigma_{cum}^2}} }
= \exp{ \frac{ \ltwo{\Delta }^2  - 2\Delta ^T (B(\u')- B^*_s) }{2\sigma_{cum}^2} },\\
&\leq \exp{ \frac{ \ltwo{\Delta }^2  + 2\Delta ^T (B(\u')- B^*_s) }{2\sigma_{cum}^2} } ,
\end{align*}
Now, $\Delta^T(B(\u')- B^*_s)$ follows $\mathcal{N}(0,\ltwo{\Delta}^2\sigma_{cum}^2 )$.  Let $\mathcal{G} =\{B^*_s | \ltwo{ \Delta^T(B(\u') - B^*_s)} \leq \ltwo{\Delta} \sigma t\}$. 

If a random variable $V\sim\mathcal{N}(0,1)$, then for all $t>1$, one has $\Pr[|V|>t]\leq e^{-t^2/2}$ ( Mill's inequality ). Thus, 
  $$\Pr [\ltwo{ \Delta^T(B(\u') - B^*_s)} \leq\ltwo{\Delta} \sigma t] \leq \exp(\frac{-t^2}{2})$$
Setting $ t= 2\sqrt{   \ln{   \frac{2\log{T}}{\delta}}        }$, we have,  with probability $1 -\frac{ \delta}{2\log{T}}$ \\
\begin{equation} \Pr [ B_{s}(\u) = B^*_{s}] \leq \exp{\frac{\epsilon}{\log{T}}}   \Pr [B_{s}(\u') = B^*_{s}]   \label{eq:2} \end{equation}

Similarly, with probability at least $1 - \frac{\delta}{2\log{T}}$ \begin{equation} \Pr [ B_{s}(\u') = B^*_{s}] \leq \exp{\frac{\epsilon}{\log{T}}}   \Pr [B_{s}(\u) = B^*_{s}]   \label{eq:1} \end{equation}
 
Using union bound with equations \eqref{eq:2} and \eqref{eq:1}, we have the claim. 
\end{proof}

Thus the proof of the theorem is now complete.
\end{proof} 
%%% Local Variables: 
%%% mode: latex
%%% TeX-master: "nips2011"
%%% End: 
